# Supplementary material for: Neurosymbolic Reinforcement Learning with Formally Verified Exploration
Source: arXiv:2009.12612 source file (2020-10-26)
Supplement: Supplementary file 1 [file sec_appendix.tex]

\appendix
\section{Appendix}
\label{sec:Appendix}
You may include other additional sections here.
